# Supplementary material for: Effect of a Temperature Gradient on the Screening Properties of Ionic Fluids
Source: arXiv:2212.12233 ancillary file (2023-04-18)
Supplement: Supplementary file 1 [file Suppl_Mat.pdf]

# Effect of a Temperature Gradient on the Screening Properties of Ionic Fluids - Supplemental Material

Andrea Grisafi[1,*] and Federico Grasselli[2,†]

[1]*PASTEUR, Département de chimie, École Normale Supérieure, PSL University, Sorbonne Université, CNRS, 75005 Paris, France*
[2]*Laboratory of Computational Science and Modeling, IMX, École Polytechnique Fédérale de Lausanne, 1015 Lausanne, Switzerland*

## DERIVATION OF THE LOCAL EQUILIBRIUM EQUATIONS

According to classical-DFT, the local equilibrium state of an inhomogeneous ionic fluid is solely determined by the ionic density distributions $\rho_{+/-}(\boldsymbol{r})$. This implies that the free-energy density in each point of the fluid can be written as a unique functional of $\rho_{+/-}(\boldsymbol{r})$. In the asymptotic regime, the density variations are assumed to be both small with respect with the reference densities $\bar{\rho}_{+/-}$ and slowly-varying with respect to the characteristic action range of the short-range correlations in the fluid [1]. In particular, an asymptotic approximation for the free-energy density of the ionic fluid can be written by virtue of a quadratic gradient expansion about $\bar{\rho}_{+/-}$:

$$f(\boldsymbol{r}) = f_0^T + \sum_i \mu_i^T \Delta\rho_i(\boldsymbol{r}) + \frac{1}{2}\sum_{ij} B_{ij}^T \Delta\rho_i(\boldsymbol{r})\Delta\rho_j(\boldsymbol{r}) + \frac{1}{2}\sum_{ij} A_{ij}^T \boldsymbol{\nabla}\rho_i(\boldsymbol{r})\cdot\boldsymbol{\nabla}\rho_j(\boldsymbol{r}) + \frac{1}{2}\rho_Q(\boldsymbol{r})\phi(\boldsymbol{r})\,, \tag{S1}$$

where $f_0^T$ and $\mu_i^T$ are the free-energy density of the chemical potentials of the homogeneous and isotropic fluid at $(\bar{\rho}_i, T)$. $\rho_Q(\boldsymbol{r}) = Z_+\rho_+(\boldsymbol{r}) + Z_-\rho_-(\boldsymbol{r})$ is the charge density, which defines the electrostatic potential as

$$\phi(\boldsymbol{r}) = \int d\boldsymbol{r}'\,\frac{\rho_Q(\boldsymbol{r}')}{|\boldsymbol{r}'-\boldsymbol{r}|}\,. \tag{S2}$$

$B_{ij}^T$ and $A_{ij}^T$ are defined as the local-density and gradient coefficients; they are respectively given by

$$B_{ij}^T = \delta_{ij}\frac{T}{\bar{\rho}_j} - 4\pi T\int_0^\infty dr\; r^2\left(c_{ij}^T(r) + \beta\frac{Z_iZ_j}{r}\right) \tag{S3}$$

and

$$A_{ij}^T(\{\bar{\rho}\}) = \frac{2\pi}{3}T\int_0^\infty dr\; r^4\left(c_{ij}^T(r) + \beta\frac{Z_iZ_j}{r}\right) \tag{S4}$$

where $c_{ij}^T(r)$ are the direct correlation functions of the reference system at $(\bar{\rho}_i, T)$.

When neglecting thermodiffusion phenomena, the local-equilibrium conditions of the system subject to a temperature distribution $T(\boldsymbol{r})$ are characterized by a vanishing isothermal gradient of the local chemical potentials [2], $\boldsymbol{\nabla}_T\mu_i(\boldsymbol{r}) = \boldsymbol{0}$. This implies that the local-equilibrium conditions can be found from the minimization of an effective non-equilibrium grand-potential at the local chemical potentials $\mu_i^T = \mu_i(T(\boldsymbol{r}))$ with respect to the ionic densities $\rho_{+/-}(\boldsymbol{r})$:

$$\frac{\delta}{\delta\rho_i(x)}\left\{F_{\mathrm{NE}}[\rho_i] - \sum_i^{+/-}\int d\boldsymbol{r}\mu_i^T\rho_i(\boldsymbol{r})\right\} = \frac{\delta F_{\mathrm{NE}}[\rho_i]}{\delta\rho_i(x)} - \mu_i^T = 0\,, \tag{S5}$$

where $F_{\mathrm{NE}}[\rho_i] \equiv \int d\boldsymbol{r} f(\boldsymbol{r})$. Assuming planar symmetry, this results in the following pair of asymptotic local-equilibrium equations for the density variations of the two ions about the reference densities $\bar{\rho}_{+/-}$:

$$0 = Z_+\phi(x) + \sum_j^{+/-} B_{+j}^T\;\Delta\rho_j(x) - \sum_j^{+/-}\frac{d}{dx}\left[A_{+j}^T\;\rho_j'(x)\right]\,, \tag{S6}$$

$$0 = Z_-\phi(x) + \sum_j^{+/-} B_{-j}^T\;\Delta\rho_j(x) - \sum_j^{+/-}\frac{d}{dx}\left[A_{-j}^T\;\rho_j'(x)\right]\,. \tag{S7}$$

Linearizing $A_{ij}^T$ and $B_{ij}^T$ about $T^0$, we obtain:

$$0 = Z_+\phi(x) + \sum_j^{+/-}\left(B_{+j}^0 + \left.\frac{\partial B_{+j}}{\partial T}\right|_0\Delta T(x)\right)\;\Delta\rho_j(x) - \sum_j^{+/-}\left[\left(A_{+j}^0 + \left.\frac{\partial A_{+j}}{\partial T}\right|_0\Delta T(x)\right)\;\rho_j''(x) + \left.\frac{\partial A_{+j}}{\partial T}\right|_0 T'(x)\rho_j'(x)\right]\,, \tag{S8}$$

$$0 = Z_- \phi(x) + \sum_j^{+/-} \left( B^0_{-j} + \left.\frac{\partial B_{-j}}{\partial T}\right|_0 \Delta T(x) \right) \Delta\rho_j(x) - \sum_j^{+/-} \left[ \left( A^0_{-j} + \left.\frac{\partial A_{-j}}{\partial T}\right|_0 \Delta T(x) \right) \rho''_j(x) + \left.\frac{\partial A_{-j}}{\partial T}\right|_0 T'(x)\rho'_j(x) \right] . \tag{S9}$$

Assuming a linear temperature variation $T(x) = T^0 + \alpha x$, these equations become

$$0 = Z_+ \phi(x) + \sum_j^{+/-} \left( B^0_{+j} + \left.\frac{\partial B_{+j}}{\partial T}\right|_0 \alpha x \right) \Delta\rho_j(x) - \sum_j^{+/-} \left[ \left( A^0_{+j} + \left.\frac{\partial A_{+j}}{\partial T}\right|_0 \alpha x \right) \rho''_j(x) + \left.\frac{\partial A_{+j}}{\partial T}\right|_0 \alpha\rho'_j(x) \right] \tag{S10}$$

$$0 = Z_- \phi(x) + \sum_j^{+/-} \left( B^0_{-j} + \left.\frac{\partial B_{-j}}{\partial T}\right|_0 \alpha x \right) \Delta\rho_j(x) - \sum_j^{+/-} \left[ \left( A_{-j} + \left.\frac{\partial A_{-j}}{\partial T}\right|_0 \alpha x \right) \rho''_j(x) + \left.\frac{\partial A_{-j}}{\partial T}\right|_0 \alpha\rho'_j(x) \right] \tag{S11}$$

Finally, we make use of the Poisson equation $\phi''(x) = -4\pi\rho_Q(x)$ to obtain a homogeneous differential system in the variables $\rho_{+/-}$

$$\begin{aligned} 0 = &-4\pi Z_+ \sum_j^{+/-} Z_j \rho_j(x) + \sum_j^{+/-} \left[ \left( B^0_{+j} + \left.\frac{\partial B_{+j}}{\partial T}\right|_0 \alpha x \right) \rho''_j(x) + 2 \left.\frac{\partial B_{+j}}{\partial T}\right|_0 \alpha\rho'_j(x) \right] \\ &- \sum_j^{+/-} \left[ \left( A^0_{+j} + \left.\frac{\partial A_{+j}}{\partial T}\right|_0 \alpha x \right) \rho''''_j(x) + 3 \left.\frac{\partial A_{+j}}{\partial T}\right|_0 \alpha\rho'''_j(x) \right] \end{aligned} \tag{S12}$$

$$\begin{aligned} 0 = &-4\pi Z_- \sum_j^{+/-} Z_j \rho_j(x) + \sum_j^{+/-} \left[ \left( B^0_{-j} + \left.\frac{\partial B_{-j}}{\partial T}\right|_0 \alpha x \right) \rho''_j(x) + 2 \left.\frac{\partial B_{-j}}{\partial T}\right|_0 \alpha\rho'_j(x) \right] \\ &- \sum_j^{+/-} \left[ \left( A^0_{-j} + \left.\frac{\partial A_{-j}}{\partial T}\right|_0 \alpha x \right) \rho''''_j(x) + 3 \left.\frac{\partial A_{-j}}{\partial T}\right|_0 \alpha\rho'''_j(x) \right] \end{aligned} \tag{S13}$$

## NUMBER AND CHARGE EQUATIONS

We are interested in writing the the previous equations in terms of the number and charge density distributions:

$$\rho_N(x) = \rho_+(x) + \rho_-(x) \qquad \rho_Q(x) = Z_+\rho_+(x) + Z_-\rho_-(x) \tag{S14}$$

Assuming for simplicity $Z_+ = -Z_- = Z$, we can then apply the change of variable

$$\rho_+(x) = \frac{1}{2}\left(\rho_N(x) + \rho_Q(x)/Z\right) \qquad \rho_-(x) = \frac{1}{2}\left(\rho_N(x) - \rho_Q(x)/Z\right) \tag{S15}$$

and consider the number and charge linear combinations of Eqs. (S12)-(S13). After doing the math, the number and charge local-equilibrium equations read as follows (we drop the suffix "0" indicating quantities at $T^0$ to lighten the notation)

$$\begin{aligned} &-\left(A_{NN} + \frac{\partial A_{NN}}{\partial T}\alpha\, x\right)\rho''''_N(x) - 3\frac{\partial A_{NN}}{\partial T}\alpha\,\rho'''_N(x) - \left(A_{NQ} + \frac{\partial A_{NQ}}{\partial T}\alpha\, x\right)\rho''''_Q(x) - 3\frac{\partial A_{NQ}}{\partial T}\alpha\,\rho'''_Q(x) \\ &+\left(B_{NN} + \frac{\partial B_{NN}}{\partial T}\alpha\, x\right)\rho''_N(x) + 2\frac{\partial B_{NN}}{\partial T}\alpha\,\rho'_N(x) + \left(B_{NQ} + \frac{\partial B_{NQ}}{\partial T}\alpha\, x\right)\rho''_Q(x) + 2\frac{\partial B_{NQ}}{\partial T}\alpha\,\rho'_Q(x) = 0 \end{aligned} \tag{S16}$$

$$\begin{aligned} &-\left(A_{QN} + \frac{\partial A_{QN}}{\partial T}\alpha\, x\right)\rho''''_N(x) - 3\frac{\partial A_{QN}}{\partial T}\alpha\,\rho'''_N(x) - \left(A_{QQ} + \frac{\partial A_{QQ}}{\partial T}\alpha\, x\right)\rho''''_Q(x) - 3\frac{\partial A_{QQ}}{\partial T}\alpha\,\rho'''_Q(x) \\ &+\left(B_{QN} + \frac{\partial B_{QN}}{\partial T}\alpha\, x\right)\rho''_N(x) + 2\frac{\partial B_{QN}}{\partial T}\alpha\,\rho'_N(x) + \left(B_{QQ} + \frac{\partial B_{QQ}}{\partial T}\alpha\, x\right)\rho''_Q(x) + 2\frac{\partial B_{QQ}}{\partial T}\alpha\,\rho'_Q(x) \\ &- 16\pi Z^2 \rho_Q(x) = 0 \end{aligned} \tag{S17}$$

where

$$A_{NN} = \sum_{ij}^{+/-} A_{ij} \qquad B_{NN} = \sum_{ij}^{+/-} B_{ij} \tag{S18}$$

$$A_{NQ} = A_{QN} = (A_{++} - A_{--}) \qquad B_{NQ} = B_{QN} = (B_{++} - B_{--}) \tag{S19}$$

$$A_{QQ} = (A_{++} + A_{--} - 2A_{+-}) \qquad B_{QQ} = (B_{++} + B_{--} - 2B_{+-}) \tag{S20}$$

When considering a symmetric salt, $A_{NQ} = B_{NQ} = 0$, and the previous equations decouple in the number and charge densities:

$$-\left(A_{NN} + \frac{\partial A_{NN}}{\partial T}\alpha\, x\right)\rho_N''''(x) - 3\frac{\partial A_{NN}}{\partial T}\alpha\,\rho_N'''(x) + \left(B_{NN} + \frac{\partial B_{NN}}{\partial T}\alpha\, x\right)\rho_N''(x) + 2\frac{\partial B_{NN}}{\partial T}\alpha\,\rho_N'(x) = 0 \tag{S21}$$

$$-\left(A_{QQ} + \frac{\partial A_{QQ}}{\partial T}\alpha\, x\right)\rho_Q''''(x) - 3\frac{\partial A_{QQ}}{\partial T}\alpha\,\rho_Q'''(x) + \left(B_{QQ} + \frac{\partial B_{QQ}}{\partial T}\alpha\, x\right)\rho_Q''(x) + 2\frac{\partial B_{QQ}}{\partial T}\alpha\,\rho_Q'(x) - 16\pi Z^2\rho_Q(x) = 0 \tag{S22}$$

## EXACT LDA CHARGE-DENSITY SOLUTIONS

For the symmetric salt, the LDA solutions for the charge distribution can be obtained by solving Eq. (S22) and imposing that $A^T_{QQ}$ vanish:

$$(a + b\,\alpha\, x)\,\rho_Q''(x) + 2\,b\,\alpha\,\rho_Q'(x) - c\,\rho_Q(x) = 0, \tag{S23}$$

where $a \equiv B^0_{QQ}$, $b \equiv \frac{\partial B_{QQ}}{\partial T}\big|_0$ and $c \equiv 16\pi Z^2$. This equation has the following exact solutions:

$$\rho_Q(x) = \frac{c}{b^2\alpha^2}\left[\frac{c(a + b\,\alpha\, x)}{b^2\alpha^2}\right]^{-1/2}\left[k_1 I_1\left(2\sqrt{\frac{c(a + b\,\alpha\, x)}{b^2\alpha^2}}\right) + k_2 K_1\left(2\sqrt{\frac{c(a + b\,\alpha\, x)}{b^2\alpha^2}}\right)\right], \tag{S24}$$

where $k_1$ and $k_2$ are constants to be determined from boundary conditions.

In case $\alpha > 0$, and if we are looking for solutions vanishing for $x \to \infty$, then only the second term must be retained, to avoid divergences, and $k_1 = 0$.

In case $\alpha < 0$, things are more subtle, since both terms vanish for $x \to \infty$. Nonetheless, for $x \geq \frac{a}{b|\alpha|}$, they become decaying oscillating functions. Notice that such condition corresponds to $B^T_{QQ} < 0$ where the LDA is no longer valid, so in principle we would lack the boundary condition on the charge density at $x \to +\infty$. This being said, from the physical point of view one should consider a monotonically decaying solution, which amount to set $k_2 = 0$ and retain only the first term. This is reported in the Mathematica notebook `LDA_exact_rho.nb`.

Thus, the asymptotic behavior of the solutions (up to constant factors determined by the boundary conditions) is:

$$\begin{cases} \rho_Q(x) \sim (a\ + b\,\alpha\, x)^{-3/4}\exp\left(-2\sqrt{\frac{c(a + b\,\alpha\, x)}{b^2\alpha^2}}\right) & \alpha > 0 \\[2ex] \rho_Q(x) \sim (a - b|\alpha|x)^{-3/4}\exp\left(+2\sqrt{\frac{c(a - b|\alpha|x)}{b^2\alpha^2}}\right) & \alpha < 0 \text{ and } x < \frac{a}{b|\alpha|} \end{cases} \tag{S25}$$

## LDA-WKB CHARGE-DENSITY SOLUTIONS

We want to show that by making use of the WKB method we can directly recover the solution in its asymptotic form. For that, let us start by applying the substitution $\rho_Q(x) = \exp(S(x))$, with $S(x)$ related to the potential of mean force of the charge density distribution. It is convenient to adopt the change of variable $y = \alpha x$ and interpreting

$\alpha$ as the WKB parameter. Doing the derivatives and simplifying the exponential everywhere we are left with the following differential equation

$$(a + by)\,\alpha^2\left[S''(y) + \left(S'(y)\right)^2\right] + 2b\alpha^2\,S'(y) - c = 0 \tag{S26}$$

Let us start considering the asymptotic expansion of $S(y)$ in increasing powers of $\alpha$ and truncate at the first order, i.e.,

$$S(y) = \frac{1}{\alpha}\sum_n \alpha^n S_n(y) \approx \frac{1}{\alpha}S_0(y) + S_1(y) + \mathcal{O}(\alpha) \tag{S27}$$

Substituting in the previous equation and keeping only the terms of order $\alpha^{n<2}$

$$(a + by)\left[\alpha S_0''(y) + \left(S_0'(y)\right)^2 + 2\alpha S_0'(y)S_1'(y)\right] + 2b\,\alpha S_0'(y) - c = 0 \tag{S28}$$

A solution for $S_0(y)$ can be found by retaining the leading order term:

$$(a + by)\left(S_0'(y)\right)^2 - c = 0 \tag{S29}$$

from which

$$S_0'(y) = \pm\sqrt{\frac{c}{a + by}} \tag{S30}$$

and finally

$$S_0(y) = \pm 2\sqrt{\frac{c(a + by)}{b^2}} + C'_\pm \tag{S31}$$

Substituting in Eq. (S28) we can now obtain an equation for $S_1(x)$:

$$\mp\,\alpha\frac{b}{2}\sqrt{\frac{c}{a + by}} + c \,\pm\, 2\alpha\sqrt{c(a + by)}S_1'(y) \,\pm\, 2b\alpha\sqrt{\frac{c}{a + bx}} - c = 0 \tag{S32}$$

from which

$$S_1'(y) = -\frac{3}{4}\frac{b}{a + by} \tag{S33}$$

and finally

$$S_1(y) = -\frac{3}{4}\log\left(a + by\right) + C' \tag{S34}$$

Putting everything together we have:

$$S(y) \approx \pm 2\sqrt{\frac{c(a + by)}{b^2\alpha^2}} - \frac{3}{4}\log\left(a + by\right) \tag{S35}$$

which yields the asymptotic solution for the charge density of Eq. (S25), q.e.d.

## SGA-WKB CHARGE-DENSITY SOLUTIONS

The solution to the complete equation cannot be found exactly, therefore we rely on the WKB method straight away. To lighten the notation we set $d \equiv -A^0_{QQ}$ and $f \equiv -\frac{\partial A_{QQ}}{\partial T}\big|_0$. After doing the derivatives, the equation for the potential of mean-force reads as follows:

$$\begin{aligned}&(d + fy)\,\alpha^4\left[\left(S'(y)\right)^4 + 4S'(y)S'''(y) + 6\left(S'(y)\right)^2 S''(y) + 3\left(S''(y)\right)^2 + S''''(y)\right]\\ &+ 3f\alpha^4\left[\left(S'(y)\right)^3 + 3S'(y)S''(x) + S'''(y)\right]\\ &+ (a + by)\,\alpha^2\left[S''(y) + \left(S'(y)\right)^2\right] + 2b\alpha^2\,S'(y) - c = 0\end{aligned} \tag{S36}$$

We once again consider the truncated asymptotic series

$$S(y)=\frac{1}{\alpha}S_0(y)+S_1(y)+\mathcal{O}(\alpha) \tag{S37}$$

Substituting and reordering in powers of $\alpha$ we obtain (c.f. the Mathematica notebook `SGA_WKB_method_complete.nb`)

$$\begin{aligned}0=&\alpha^0\Big[(a+by)[S_0'(y)]^2-c+(d+fy)[S_0'(y)]^4\Big]\\&+\alpha^1\Big[(a+by)\left[S_0''(y)+2S_0'(y)S_1'(y)\right]+2bS_0'(y)+(d+fy)\left[4[S_0'(y)]^3S_1'(y)+6[S_0'(y)]^2S_0''(y)\right]+3f[S_0'(y)]^3\Big]\\&+\mathcal{O}(\alpha^2).\end{aligned} \tag{S38}$$

By taking the leading order we get:

$$(d+fy)\left[S_0'(y)\right]^4+(a+by)\left[S_0'(y)\right]^2-c=0 \tag{S39}$$

from which we have the four solutions

$$S_{0_{1,2}}'(y)=\mp\sqrt{-\frac{(a+by)+\sqrt{(a+by)^2+4c\,(d+fy)}}{2\,(d+fy)}}\,,\qquad S_{0_{3,4}}'(y)=\mp\sqrt{\frac{-\,(a+by)+\sqrt{(a+by)^2+4c\,(d+fy)}}{2\,(d+fy)}} \tag{S40}$$

and finally $S_{0_{1,2,3,4}}(y)$ from direct integration, which we performed with Wolfram Mathematica. These four solutions are analytical, but quite byzantine, and are not reported here. The interested reader can find the explicit form of $S_{0_{1,2,3,4}}(y)$ in the supplemental notebook `SGA_WKB_method_complete.nb`.

By considering all the needed derivatives of $S_0(y)$ and substituting the solutions just found into the second line of Eq. (S38), we can now solve for $S_1'(y)$:

$$S_1'(y)=-\frac{2bS_0'(y)+3f\left[S_0'(y)\right]^3+(a+by)\,S_0''(y)+6(d+fy)\left[S_0'(y)\right]^2S_0''(y)}{4\,(d+fy)\left[S_0'(y)\right]^3+2(a+by)S_0'(y)} \tag{S41}$$

to obtain $S_1$ associated to the first pair, $S_{0_{1,2}}$

$$\begin{aligned}S_1(y)=\frac{1}{4}\Big\{&-\log[d+fy]\\&-\log\Big[(a+by)^2+4c(d+fy)\Big]\\&+\frac{1}{2}\log\Big[ab+2cf+b^2y+b\sqrt{(a+by)^2+4c(d+fy))}\Big]\\&+\frac{1}{2}\log\Big[-abd+a^2f+2cdf+(abf-b^2d+2cf^2)\,y+(af-bd)\sqrt{(a+by)^2+4c(d+fy)}\Big]\Big\}\end{aligned} \tag{S42}$$

and to the second pair $S_{0_{3,4}}$:

$$\begin{aligned}S_1(y)=\frac{1}{4}\Big\{&-\log[(a+by)^2+4c(d+fy)]\\&-\frac{1}{2}\log\Big[ab+2cf+b^2y+b\sqrt{(a+by)^2+4c(d+fy)}\Big]\\&-\frac{1}{2}\log\Big[-abd+a^2f+2cdf+(abf-b^2d+2cf^2)y+(af-bd)\sqrt{(a+by)^2+4c(d+fy)}\Big]\Big\}.\end{aligned} \tag{S43}$$

## CHARGE DENSITY INTEGRALS

We report here the analytical expression for the charge integral of the LDA/WKB solutions from the position of the surface $x = 0$, of charge density $\eta$, to a given point $x$ in the fluid:

$$Q(x) = \int_0^x dx' \, \rho_Q(x') = -\eta + C_Q \, \Gamma \left[ \frac{1}{2}, 2\sqrt{\frac{c\,(a + b\alpha x)}{b^2 \alpha^2}} \right] , \tag{S44}$$

with $\Gamma$ the Gamma-function and $C_Q$ a constant to be determined from boundary conditions. The asymptotic behaviour of the residual charge (second term at r.h.s.) can be related to the capability of the fluid to perfectly screen an external charge. In particular, when taking the limit of $x \to \infty$ we get

$$Q(x) + \eta \sim x^{-\frac{1}{4}} \exp\left( -2\sqrt{\frac{c}{b\alpha} x} \right) . \tag{S45}$$

We recognize that this expression goes to zero faster than the problem dimensionality $x$, thus guaranteeing the perfect screening of an external charge over a finite distance.

For completeness, in Fig. S1 we also report the dependence of the integrated charge with respect to the temperature gradient $\alpha$ for the parameters of Sec. III D of the main text.

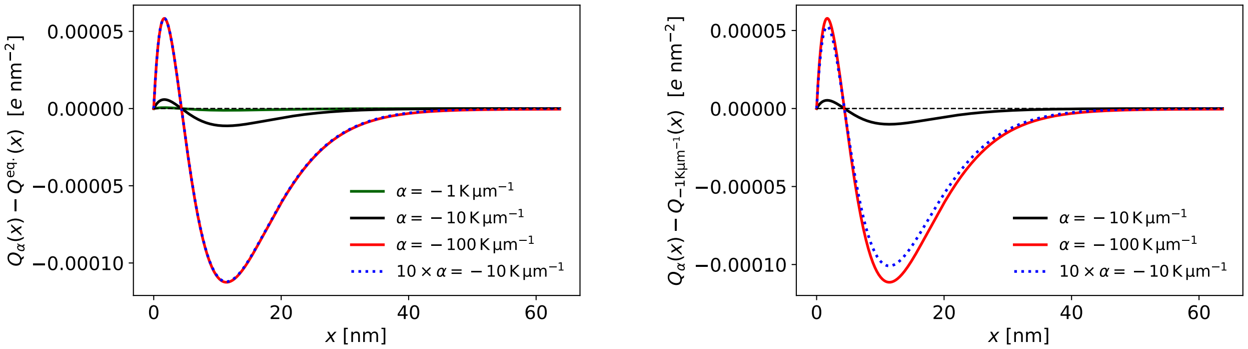


FIG. S1. (Left) Difference between the integrated charge functions of the LDA/WKB solution and of the equilibrium DH solution, at different temperature gradients, $\alpha$. The dotted blue line indicates 10 times the red curve, and well superimposes to the latter, as described in Sec. III D of the main manuscript. (Right) Difference between the integrated charge functions of the LDA/WKB solution at a given $\alpha$ with that at $\alpha = -1$ K $\mu$m$^{-1}$. The dotted blue line indicates 10 times the red curve. Here no superimposition occurs.

We finally report, in Fig. S2 the deviation from equilibrium of the integrated charge density in the SGA approximation.

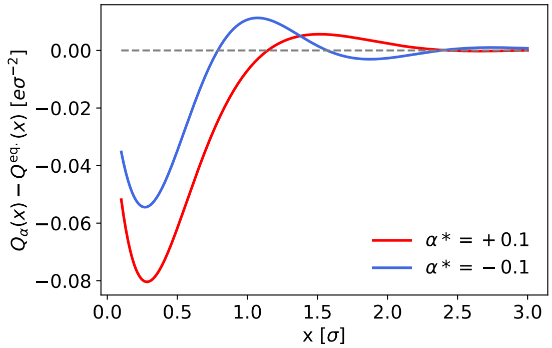


FIG. S2. Difference between the integrated charge functions of the SGA/WKB solution and of the equilibrium DH solution, at different temperature gradients , $\alpha = \alpha^* T^0/\sigma$, with $T^0 = 500\epsilon$.

## LINEAR SCALE CHARGE-DENSITY PROFILES

We report below the linear-scale LDA and SGA charge-density screening profiles associated with Figs.2 and 3 of the main text, respectively. Note that the non-monotonic behavior of the SGA solutions in the vicinity of the surface

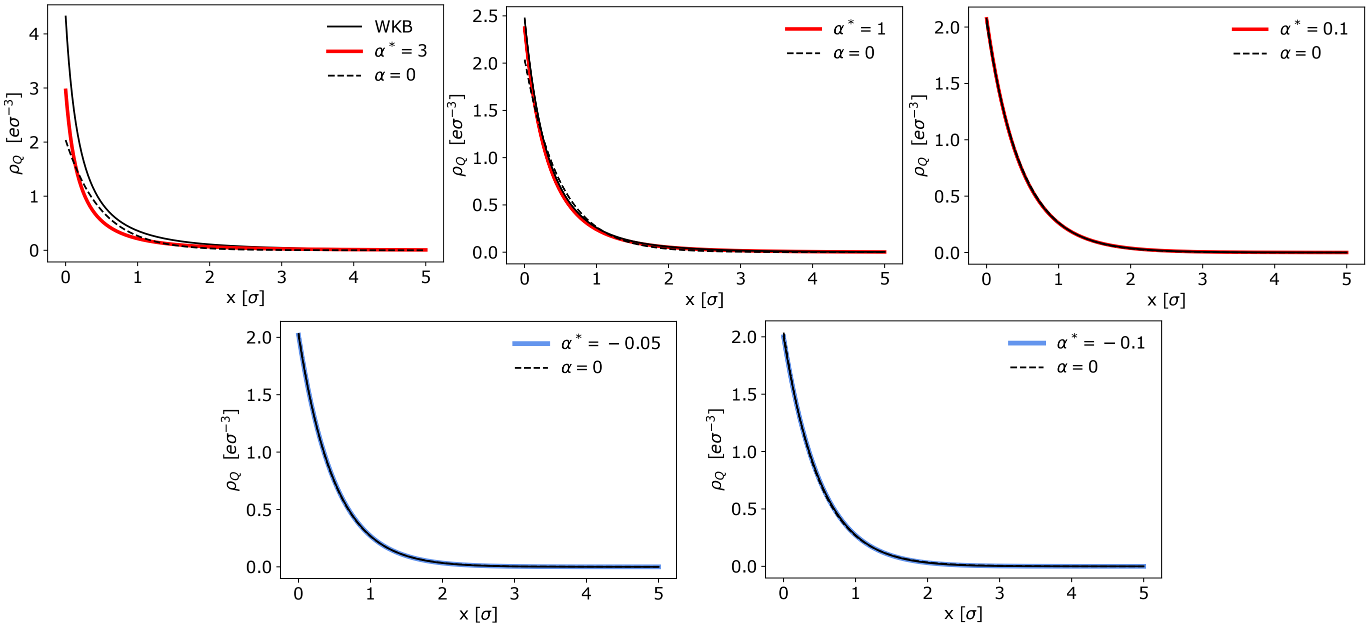


FIG. S3. Linear-scale LDA screening profiles for different temperature gradients $\alpha^* = \alpha/T^0$.

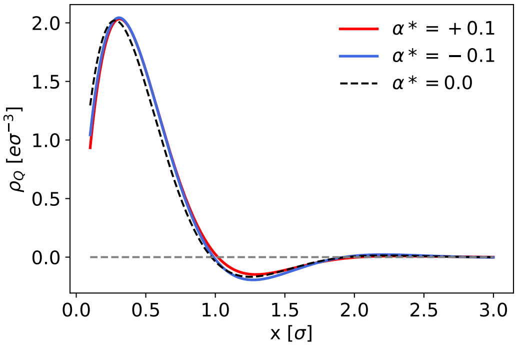


FIG. S4. Linear-scale SGA screening profiles for different temperature gradients $\alpha^* = \alpha/T^0$.

reflects the approximate nature of the free-energy functional which has been derived in order to accurately describe the asymptotic screening profile at sufficiently small and slowly varying charge-density variations. In contrast, we observe that the underlying rigidity of the LDA solutions yields charge-density profiles that appear as more physical in the proximity of charged surface.

## ELECTROSTATIC POTENTIAL

Once solutions for the charge density are found, the electrostatic potential can be extracted from Eq.9 as:

$$\phi(x) = -\frac{1}{4Z^2}\left\{B^T_{QQ}\rho_Q(x) - \frac{d}{dx}\left[A^T_{QQ}\,\rho'_Q(x)\right]\right\}, \tag{S46}$$

We report below the result for the LDA and SGA solutions associated with Fig. 2 and 3 of the main text. We observe that the asymptotic behaviour of $\phi$ mirrors that of $\rho_Q$.

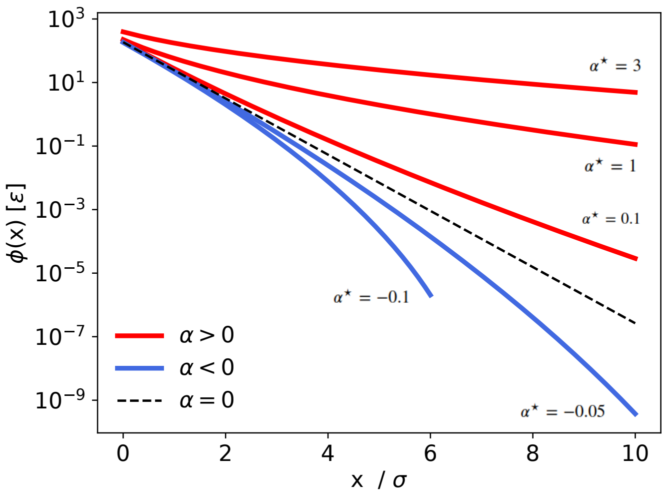


FIG. S5. Asymptotic behaviour of the LDA electrostatic potential for different temperature gradients $\alpha^* = \alpha/T^0$.

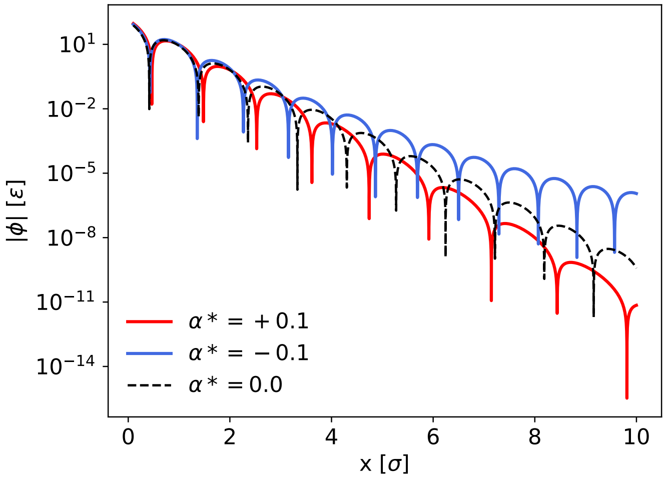


FIG. S6. Asymptotic behaviour of the SGA electrostatic potential for different temperature gradients $\alpha^* = \alpha/T^0$.

## CALCULATION OF LOCAL-DENSITY AND GRADIENT COEFFICIENTS

The local-density and square-gradient coefficients of the reference system at $T^0$ can be computed as follows:

$$B_{ij}^0 = \delta_{ij}\frac{T^0}{\bar{\rho}_j} - 4\pi T^0 \int_0^\infty dr\, r^2 \left( c_{ij}^0(r) + \beta \frac{Z_i Z_j}{r} \right) \tag{S47}$$

and

$$A_{ij}^0(\{\bar{\rho}\}) = \frac{2\pi}{3} T^0 \int_0^\infty dr\, r^4 \left( c_{ij}^0(r) + \beta \frac{Z_i Z_j}{r} \right) \tag{S48}$$

where $c_{ij}^0(r)$ are the direct correlation functions of the reference system at $(\bar{\rho}_i, T^0)$. These are computed using the hypernetted chain (HNC) closure to the Ornstein-Zernike equation [3]. For that, we rely on an efficient code that is implemented following the algorithm reported in Ref. [4]. From the previous definitions, the derivative of the parameters with respect to temperature are computed by finite differences. In Fig. S7, we report the behaviour of $A_{QQ}^T$ and $B_{QQ}^T$ as a function of the temperature $T$: while the $B_{QQ}^T$ parameters shows a linear behaviour over a broad range of temperatures, the dependence of $A_{QQ}^T$ from $T$ can be approximated with a line only over a reduced temperature window.

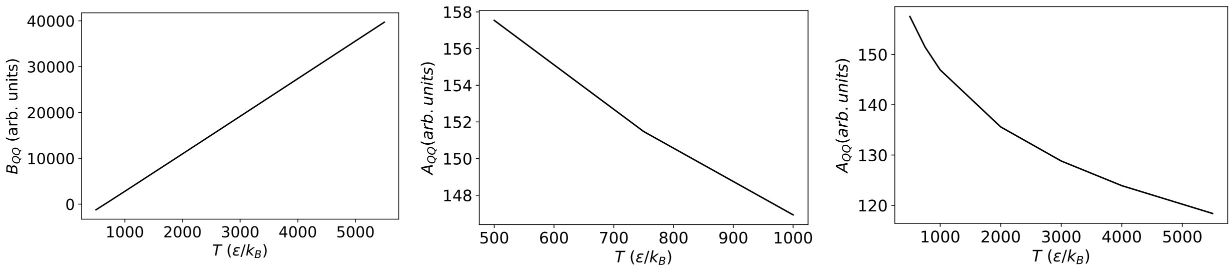


FIG. S7. Temperature dependence of the $B^T_{QQ}$ and $A^T_{QQ}$ parameters computed at the reference number density $\bar{\rho}_N = 0.5$ ions/$\sigma^3$ using the HNC approximation.

## LOCATION OF THE LOCAL CROSSOVER TEMPERATURE

We report below a comparison of the oscillatory to monotonic structural crossover of the charge-density decay for reference temperature values $T^0$ that are closer and closer to the expected crossover temperature $T^*$ of the equilibrium system at the reference density $\bar{\rho}_N$. We observe a vanishing discrepancy between the location of the cusp predicted by our WKB solutions and the expected location of $T^*$ for $T^* \to T^0$. This behavior can be attributed to the fact that the adopted linear approximation of $A^T_{QQ}$ about $T^0$ is increasingly good for $T(x) \to T^0$, while non-linear approximations of $A^T_{QQ}$ would be in general better suited for values of $x$ far from $x = 0$.

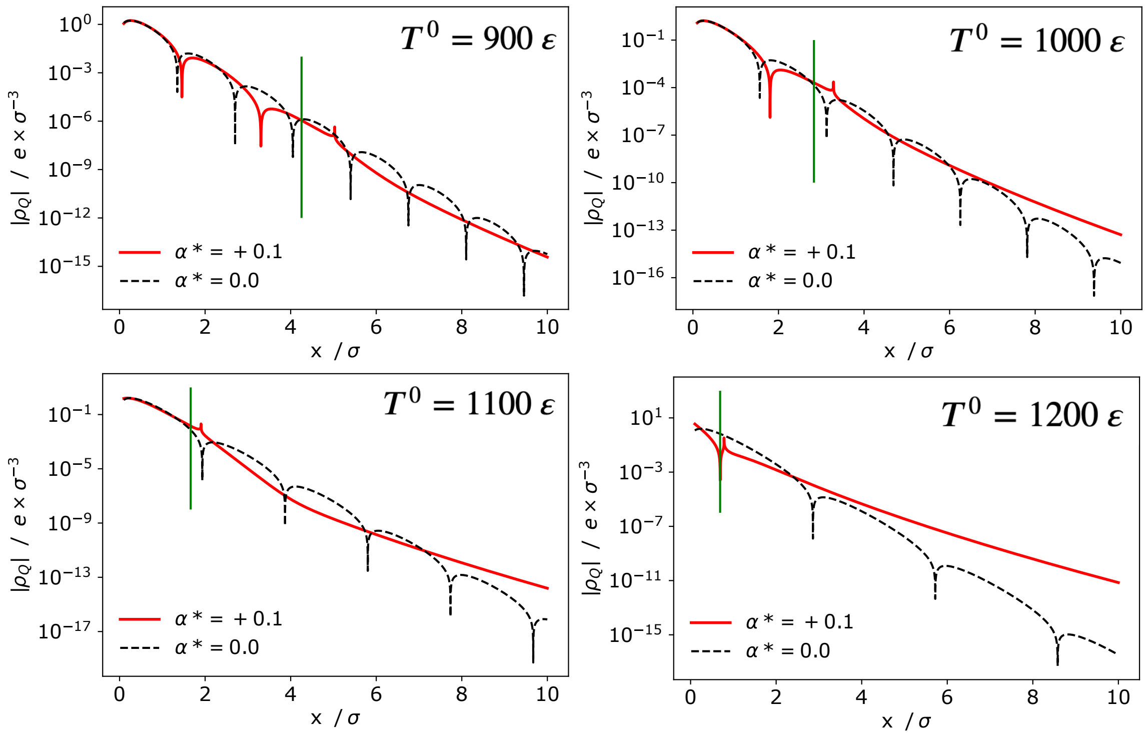


FIG. S8. Oscillatory to monotonic structural crossover of the SGA/WKB solutions for the charge-density decay under a temperature gradient $\alpha = \alpha^* T^0$, reported for different values of the reference temperature $T^0$ corresponding to the local temperature at $x = 0$. Green vertical line: expected location of the crossover temperature $T^* = 1285\,\varepsilon$ as predicted from the Fisher-Widom line of the thermal equilibrium system at the reference density $\bar{\rho}_N = 0.5\,\text{ions} \times \sigma^{-3}$.

## DILUTE ELECTROLYTE BETWEEN CHARGED WALLS

We report below the charge density distributions and deviation of the electrostatic potential with respect to the DH equilibrium results at $T^0$ =300K for the dilute electrolyte model of ionic density $\bar{\rho}_N = 0.01$M under a stationary temperature gradient of $\alpha = -10$K/$\mu$m, embedded between two oppositely charged walls of surface charge density $\eta = \pm 1e/\text{nm}^2$.

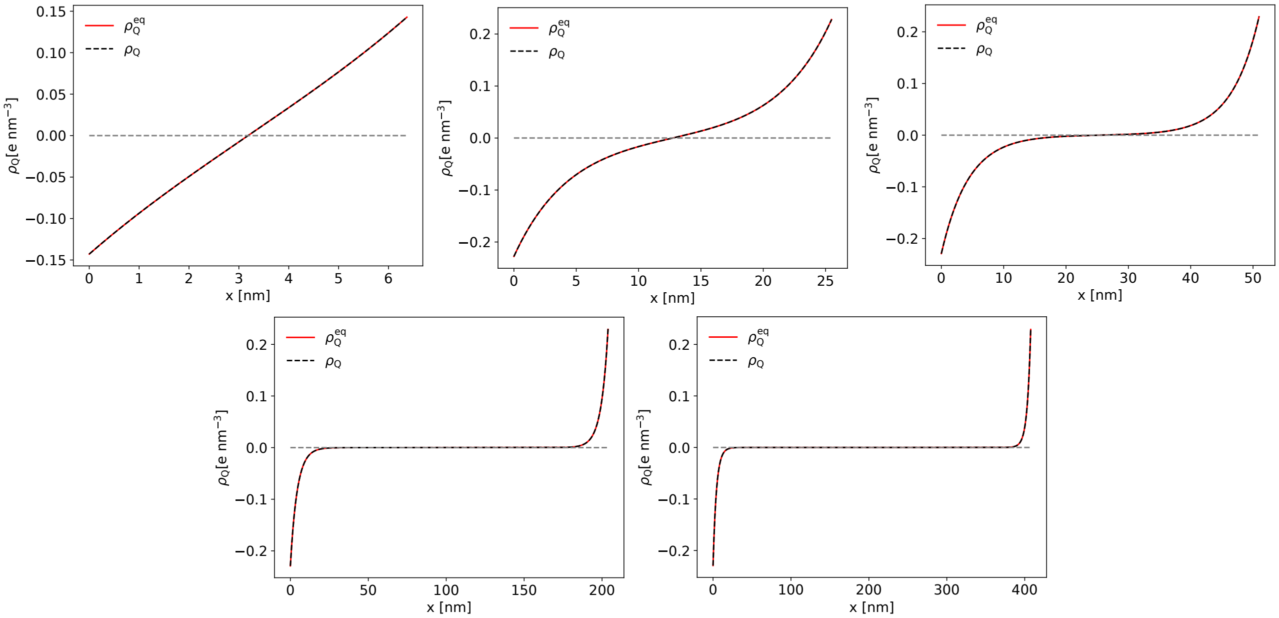


FIG. S9. Charge density distribution of a dilute electrolytes solution embedded between two oppositely charged walls, reported as a function of the walls reciprocal distance $L$. Red lines: equilibrium DH profiles. Black dashed lines: non-equilibrium LDA profiles, reported for different distances between the two walls.

We also report below the electrostatic potential drop predicted by the equilibrium DH model at $T^0$, as a function of the reciprocal distance between the two walls.

* andrea.grisafi@ens.psl.eu
† federico.grasselli@epfl.ch
[S1] P. D. Fleming III, A. J. M. Yang, and J. H. Gibbs, J. Chem. Phys. **65**, 7 (1976).
[S2] S. de Groot and P. Mazur, *Non-equilibrium Thermodynamics*, Dover Books on Physics (Dover Publ., 1984).
[S3] J.-P. Hansen and I. R. McDonald, *Theory of Simple Liquids*, 4th ed. (Academic Press, Oxford, 2013).
[S4] G. Abernethy and M. Gillan, Mol. Phys. **39**, 839 (1980).

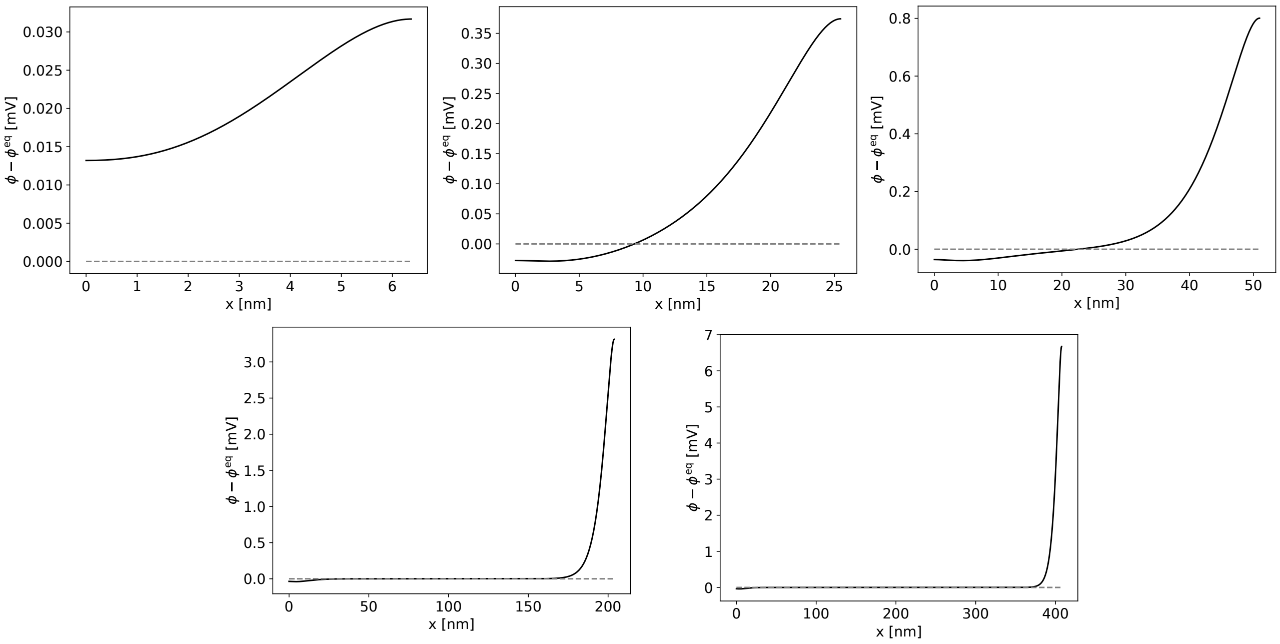


FIG. S10. Deviation of the electrostatic potential predicted by the non-equilibrium solutions with respect to the DH equilibrium results for a dilute electrolyte solution embedded between two oppositely charged walls, reported for different distances between the two walls.

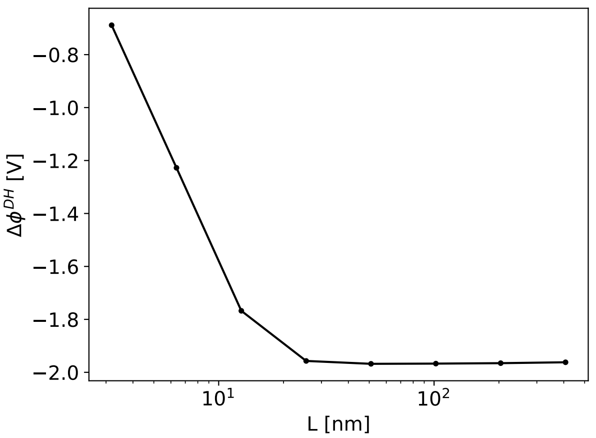


FIG. S11. Electrostatic potential drop between the two walls derived from the equilibrium DH solutions at the reference temperature $T^0$, reported as a function of the walls reciprocal distance $L$.
